# Supplementary material for: Robust Global Structure-from-Motion via View Graph Pruning
Source: arXiv:2608.22054 source file (2026-08-22)
Supplement: Supplementary file 1 [file X_suppl.tex]

\clearpage
\setcounter{section}{0}
\setcounter{figure}{0}
\setcounter{table}{0}
\setcounter{page}{1}
\renewcommand\thesection{\Alph{section}}
\renewcommand\thetable{\Alph{table}}
\renewcommand\thefigure{\Alph{figure}}
\maketitlesupplementary

% 使用的配置是 

\section{Hardware Information}  
\label{sec:imp}

All our experiments and computational time comparisons are conducted on a personal computer equipped with an AMD EPYC 7542 32-core CPU and an RTX A6000 GPU. Similar to COLMAP~\cite{schoenberger2016sfm}, our method uses the GPU solely for feature extraction and matching..

\section{Additional Experiments}  
\label{sec:add_exp}

We report additional experiments comparing our method with GLOMAP~\cite{pan2024glomap}, COLMAP~\cite{schoenberger2016sfm}, GraphSfM~\cite{chen2020graph}, Doppelgangers~\cite{cai2023doppelgangers}, and Doppelgangers++~\cite{xiangli2025doppelgangers++}.

\subsection{Evaluation on Sequential Datasets}

% 第二个实验测试的是顺序的数据集 用到的数据是Family Auditorium Courthouse Meetingroom 
% 来自论文A. Knapitsch, J. Park, Q.-Y. Zhou, and V. Koltun, “Tanks and temples:
% Benchmarking large-scale scene reconstruction,” ACM Trans. Graph.,
% vol. 36, no. 4, pp. 1–13, Jul. 2017.
% 我们自己拍摄的数据 花坛 图书馆 花坛 花坛
% 对比的方法有glomap colmap xrsfm graphsfm 

In Fig.~\ref{fig:cmp4}, we report the  qualitative comparisons on sequential image datasets from the Tanks and Temples benchmark~\cite{knapitsch2017tanks}. Specifically, we provide results on the dataset ``Family'', ``Auditorium'', ``Courthouse'' and ``Meetingroom''. On these datasets, both our method and the comparison methods yield plausible results. However, as indicated by the red arrow in Fig.~\ref{fig:cmp4}, compared to Doppelgangers++~\cite{xiangli2025doppelgangers++}, which has some missing registered cameras, our camera trajectory is more complete.

\begin{figure*}[h]
\centering
\includegraphics[width=1.0\linewidth]{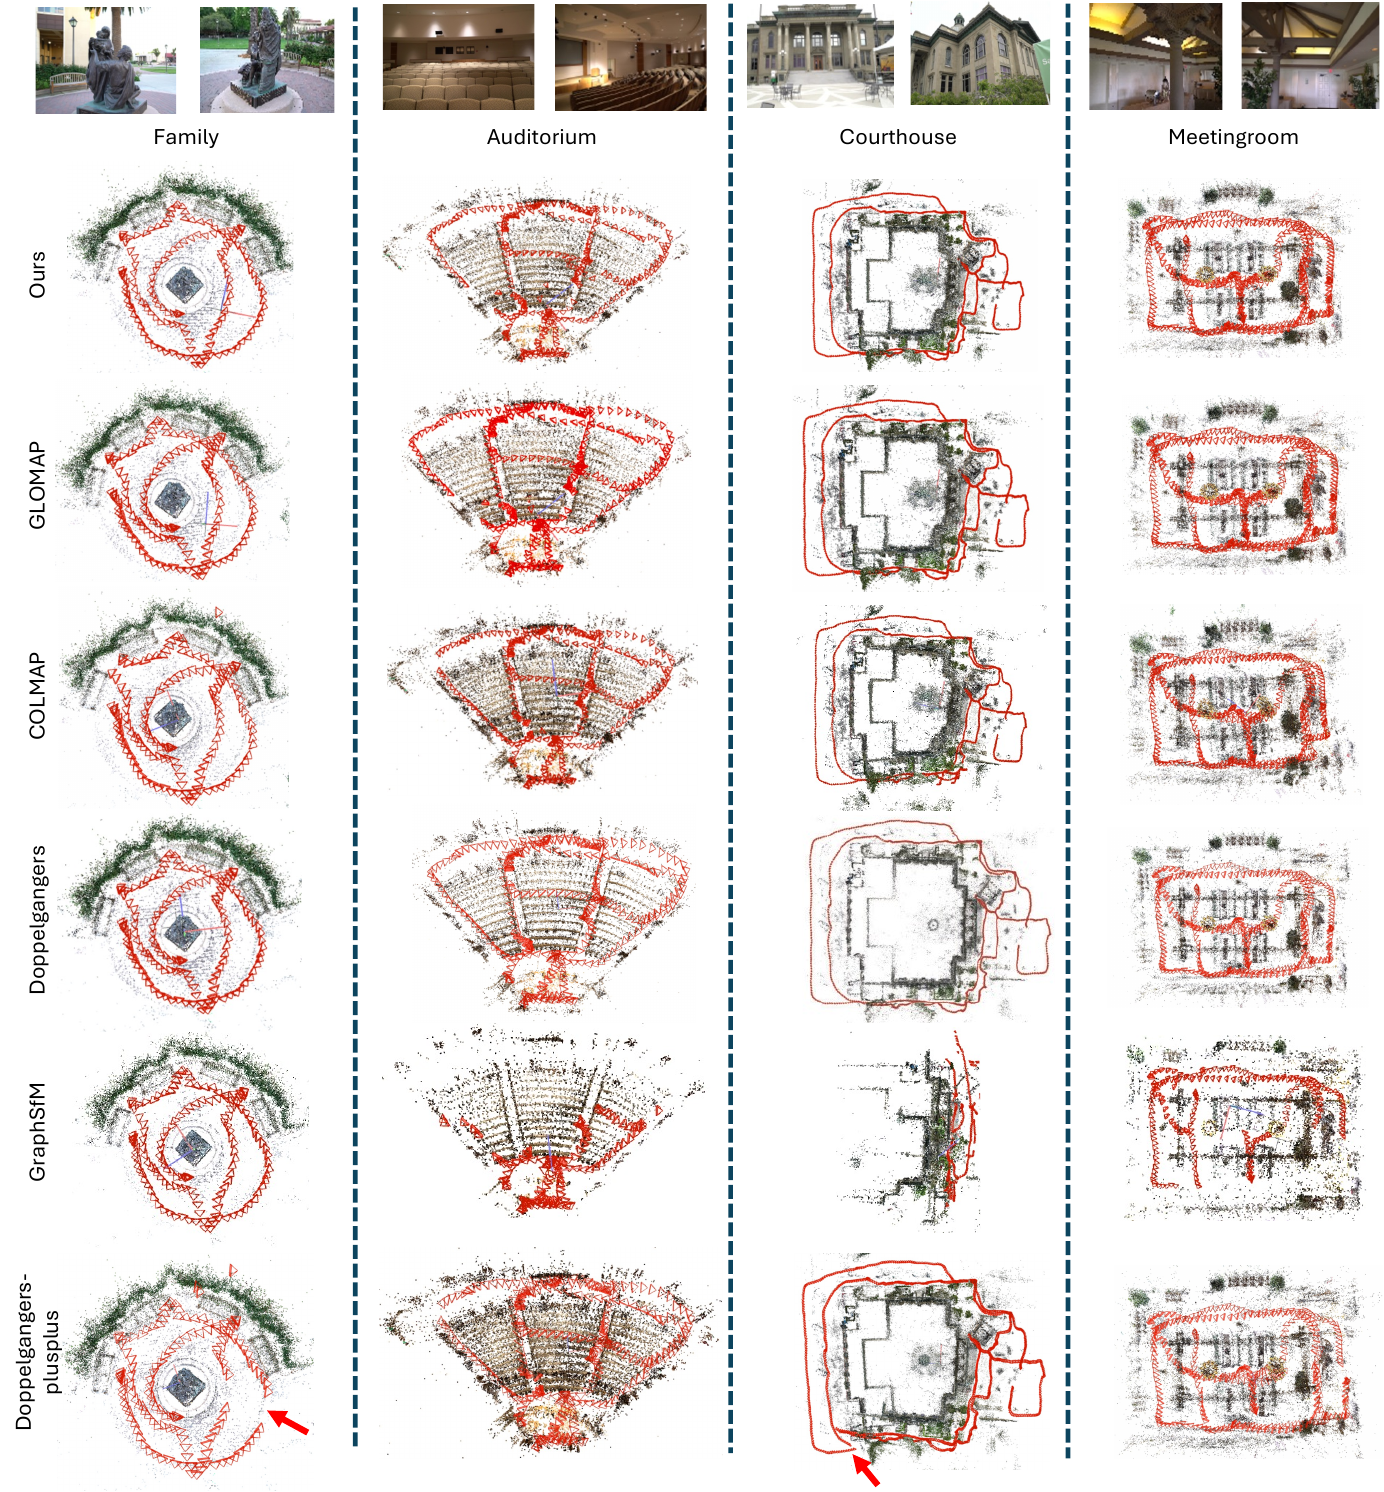}
\caption{Qualitative evaluation on the Tanks and Temples benchmark~\cite{knapitsch2017tanks}.}
\label{fig:cmp4} 
\end{figure*}

\subsection{Evaluation on Unordered Internet Image Datasets}
% 第三个实验测试的是Unordered Internet Image 数据indoor 
% 来自N. Jiang, P. Tan, and L.-F. Cheong, “Seeing double without confusion:
% Structure-from-motion in highly ambiguous scenes,” in Proc. IEEE Conf.
% Comput. Vis. Pattern Recognit., Jun. 2012, pp. 1458–1465.
% 数据 Brandenburg Gate， Arc de Triomphe 
% 来自 J. Heinly, E. Dunn, and J. M. Frahm, “Correcting for duplicate scene
% structure in sparse 3D reconstruction,” in Proc. Eur. Conf. Comput. Vis.
% Cham, Switzerland: Springer, 2014, pp. 780–795.
% 对比的方法有glomap colmap graphsfm 

In Fig.~\ref{fig:cmp3}, we present qualitative comparisons on the unordered Internet image datasets~\cite{heinly2014correcting}. Compared to GLOMAP~\cite{pan2024glomap}, COLMAP~\cite{schoenberger2016sfm}, Doppelgangers~\cite{cai2023doppelgangers}, and Doppelgangers++~\cite{xiangli2025doppelgangers++}, our reconstruction results are more accurate. As shown in Fig.~\ref{fig:cmp3}, both GLOMAP~\cite{pan2024glomap} and COLMAP~\cite{schoenberger2016sfm} exhibit large missing areas in the ``indoor'' dataset~\cite{jiang2012seeing} and the ``Arc de Triomphe'' dataset~\cite{heinly2014correcting}. While Doppelgangers++~\cite{xiangli2025doppelgangers++} achieve better results, we can observe from the parallel walls in the ``Arc de Triomphe'' dataset~\cite{heinly2014correcting} that the accuracy of our method is superior.

\begin{figure*}[h]
\centering
\includegraphics[width=0.8\linewidth]{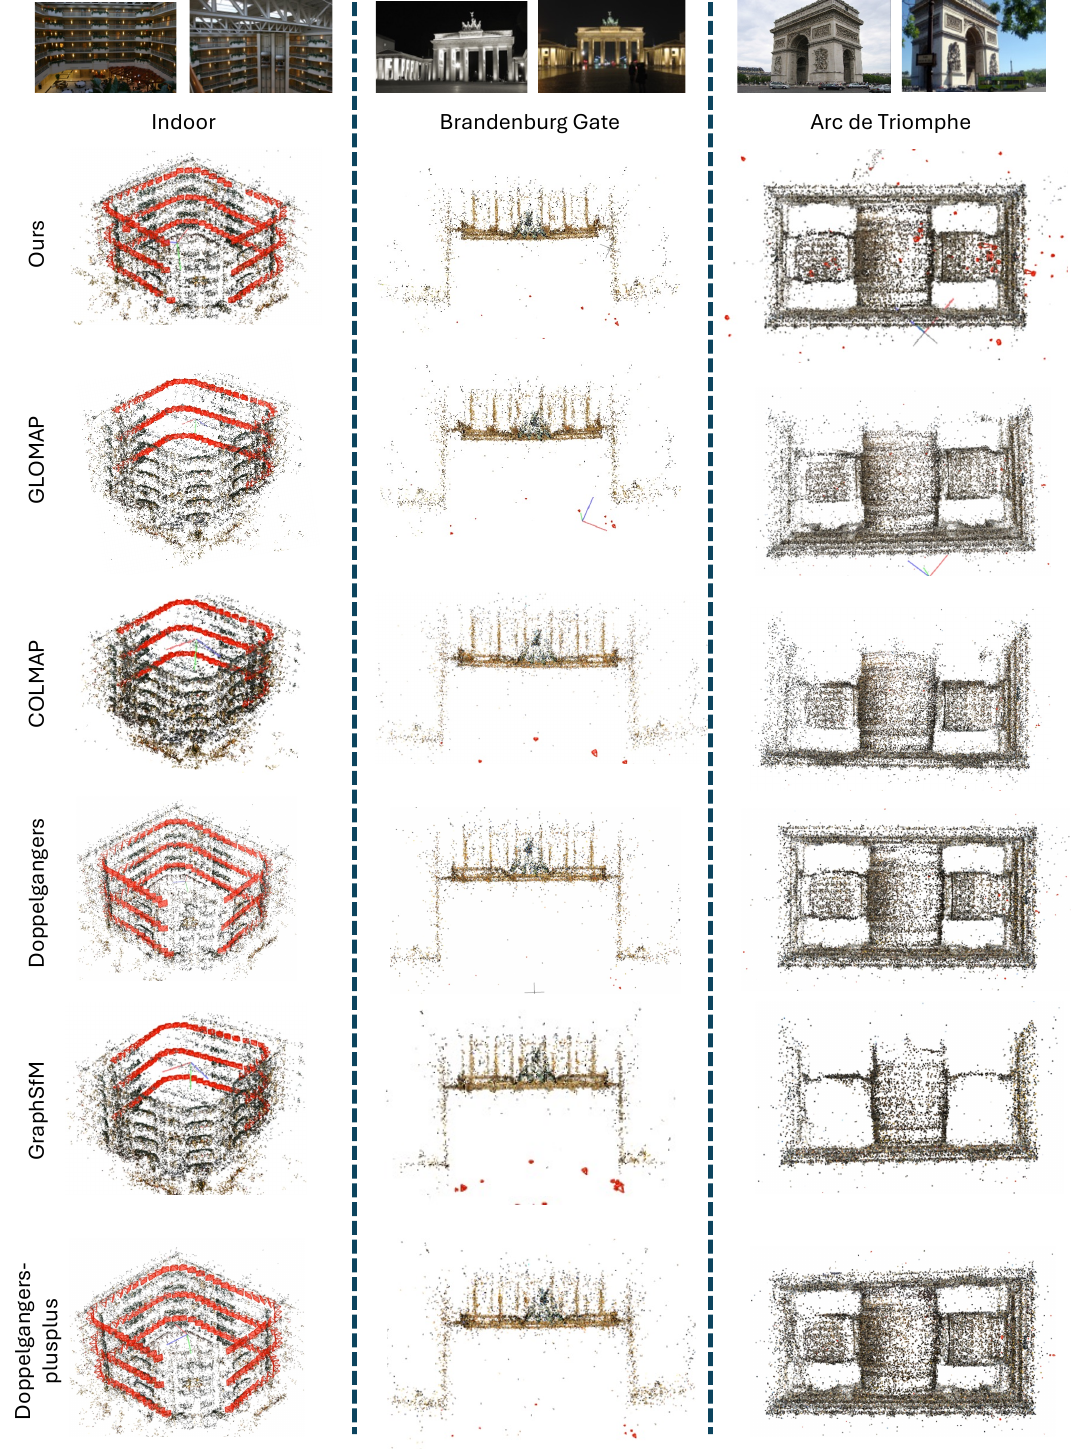}
\caption{Qualitative evaluation on Unordered Internet Image Datasets.}
\label{fig:cmp3} 
\end{figure*}

\begin{figure*}[h]
\centering
\includegraphics[width=0.8\linewidth]{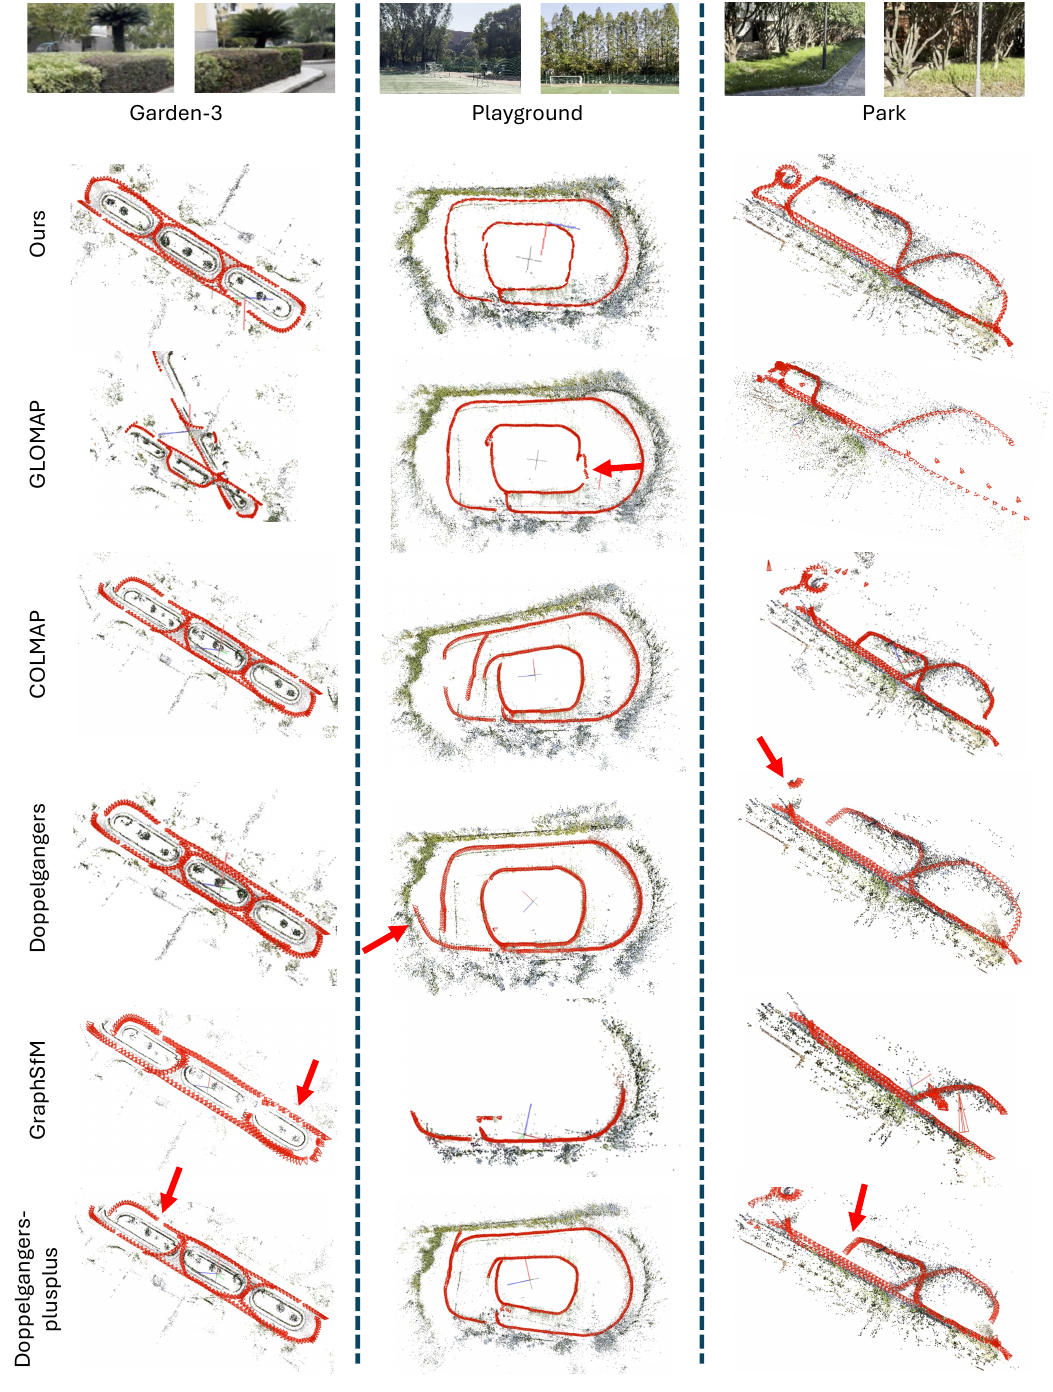}
\caption{Qualitative evaluation on additional captured scenes.}
\label{fig:cmp5} 
\end{figure*}

\subsection{Additional Evaluation on Our Captured Datasets}

We evaluate our method on additional captured scenes, namely ``Garden-3'', ``Playground'', and ``Park'', as shown in Fig.~\ref{fig:cmp5}. For all three scenes, our method achieves the best results. Note that all three datasets contain distinct areas with visual similarity, which can cause ambiguity during SfM reconstruction. In the case of vanilla GLOMAP~\cite{pan2024glomap} (Row 2), the trajectory is incorrect for ``Garden-3'' and ``Park'', and there is also misalignment in the ``Playground'' scene. Similarly, COLMAP and GraphSfM fail to reconstruct the complete scenes. The learning-based methods, Doppelgangers~\cite{cai2023doppelgangers} and the more recent Doppelgangers++~\cite{xiangli2025doppelgangers++}, are better at handling some ambiguities compared to GLOMAP~\cite{pan2024glomap}, but still suffer from local misalignment, as indicated by the red arrow.
